# Supplementary material for: Test Coverage for Network Configurations
Source: arXiv:2209.12870 source file (2022-09-26)
Supplement: Supplementary file 1 [file datamodel.tex]

%\section{IFG data model}

\begin{figure*}
\begin{tabular}{l|lr|l}
\toprule
\textbf{Node type}& \textbf{Data attributes} & & \textbf{Explanation}

\\ \midrule
\multirow{5}{*}{Main RIB entry}
& \py{host} & \py{str} & Name of router (or VRF) who owns this entry
\\ \cline{2-4}
& \py{prefix} & \py{str} & Destination subnet
\\ \cline{2-4}
& \py{nexthop} & \py{str} & Next hop IP address or interface
\\ \cline{2-4}
& \py{protocol} & \py{str} & Source routing protocol of this entry
\\ \cline{2-4}
& \py{admin_dist} & \py{int} & Administrative distance

\\ \hline
\multirow{3}{*}{Connected RIB entry}
& \py{host} & \py{str} & Name of router (or VRF) who owns this 
\\ \cline{2-4}
& \py{prefix} & \py{str} & Destination subnet
\\ \cline{2-4}
& \py{nexthop_interface} & \py{str} & Output interface

\\ \hline
\multirow{7}{*}{BGP RIB entry}
& \py{host} & \py{str} & Name of router (or VRF) who owns this entry
\\ \cline{2-4}
& \py{prefix} & \py{str} & Destination subnet
\\ \cline{2-4}
& \py{nexthop_ip} & \py{str} & Next hop IP address
\\ \cline{2-4}
& \py{as_path} & \py{List[List[int]]} & AS path
\\ \cline{2-4}
& \py{communities} & \py{List[int]} & Community tags
\\ \cline{2-4}
& \py{localpref} & \py{int} & Local preference
\\ \cline{2-4}
& \py{is_best} & \py{bool} & Whether this entry is selected as a best route

\\ \hline
\multirow{7}{*}{BGP message}
& \py{send_host} & \py{str} & Name of router (or VRF) who sends this message
\\ \cline{2-4}
& \py{recv_host} & \py{str} & Name of router (or VRF) who receives this message
\\ \cline{2-4}
& \py{prefix} & \py{str} & Destination subnet
\\ \cline{2-4}
& \py{nexthop_ip} & \py{str} & Next hop IP address
\\ \cline{2-4}
& \py{as_path} & \py{List[List[int]]} & AS path
\\ \cline{2-4}
& \py{communities} & \py{List[int]} & Community tags
\\ \cline{2-4}
& \py{is_pre_import} & \py{str} & Whether this message is pre-import or post-import

\\ \hline
\multirow{8}{*}{BGP edge}
& \py{send_host} & \py{str} & End router (or VRF) of this BGP session who sends messages
\\ \cline{2-4}
& \py{recv_host} & \py{str} & End router (or VRF) of  this BGP session who receives messages
\\ \cline{2-4}
& \py{send_ip} & \py{str} & Sender's IP address for this BGP session
\\ \cline{2-4}
& \py{recv_ip} & \py{str} & Receiver's IP address for this BGP session
\\ \cline{2-4}
& \py{send_as} & \py{int} & Sender's AS number
\\ \cline{2-4}
& \py{recv_as} & \py{int} & Receiver's AS number
\\ \cline{2-4}
& \py{export_policy} & \py{List[str]} & A sequence of routing policies at sender's export
\\ \cline{2-4}
& \py{import_policy} & \py{List[str]} & A sequence of routing policies at receiver's import

\\ \hline
\multirow{1}{*}{Path}
& \py{-} & \py{-} & TBA

\\ \hline
\multirow{4}{*}{Interface config}
& \py{host} & \py{str} & Name of router who owns this config
\\ \cline{2-4}
& \py{name} & \py{str} & Name of interface
\\ \cline{2-4}
& \py{prefix} & \py{str} & Assigned subnet
\\ \cline{2-4}
& \py{lines} & \py{List[int]} & Line numbers of this element in the configuration file

\\ \hline
\multirow{5}{*}{BGP peer config}
& \py{host} & \py{str} & Name of router who owns this config
\\ \cline{2-4}
& \py{remote_as} & \py{int} & AS number of peer
\\ \cline{2-4}
& \py{remote_ip} & \py{str} & IP address of peer
\\ \cline{2-4}
& \py{peer_group} & \py{str} & Peer group that this peer belongs to
\\ \cline{2-4}
& \py{lines} & \py{List[int]} & Line numbers of this element in the configuration file

\\ \hline
\multirow{4}{*}{Routing policy term}
& \py{host} & \py{str} & Name of router who owns this config
\\ \cline{2-4}
& \py{policy} & \py{str} & Routing policy that this term belongs to
\\ \cline{2-4}
& \py{seq} & \py{str} & Identifier (name or sequence number) of this term
\\ \cline{2-4}
& \py{lines} & \py{List[int]} & Line numbers of this element in the configuration file

\\ \bottomrule
\end{tabular}
\caption{IFG data model.}
\label{fig:datamodel}
\end{figure*}
