# Supplementary material for: Test Coverage for Network Configurations
Source: arXiv:2209.12870 source file (2022-09-26)
Supplement: Supplementary file 2 [file primitives.tex]

%\section{IFG data model}

\begin{figure*}
\begin{tabular}{l|l}
\toprule
\textbf{Primitive} & \textbf{Explanation}

\\ \midrule
\py{lookup(**kwargs)}  & -

\\ \midrule
\py{policy_evaluation(input_route, policy)}  & -

\\ \midrule
\py{longest_prefix_match(input_rib, ip)}  & -

\\ \midrule
\py{traceroute(start_location, src_ip, dst_ip, src_port, dst_port, ip_protocol)}  & -

\\ \bottomrule
\end{tabular}
\caption{Primitives used by inference rules}
\label{fig:primitives}
\end{figure*}
