# Supplementary material for: Test Coverage for Network Configurations
Source: arXiv:2209.12870 source file (2022-09-26)
Supplement: Supplementary file 3 [file rules.tex]

\section{Inference Rules}\label{appendix:rules}

\para{Given main RIB route, infer its incoming edge from parent BGP route}
%\begin{figure}[h]
 \begin{minted}[breaklines,linenos,fontsize=\small]{python}
def infer_main_route_from_bgp_route(r, input_facts):
  parent = input_facts.bgp_rib_entries.lookup(
    host=r.host,
    prefix=r.prefix,
    nexthop=r.nexthop,
    status='BEST'
  )
  return [(r, parent)]
 \end{minted}
%\caption{Infer RIB entries that led to a FIB entry.}
%\end{figure}

\para{Given main RIB route, infer its incoming edge from another main RIB route that resolves its next hop IP address} This process can be recursive, \EG, when an BGP route depends on an OSPF route to resolve the ip address to the iBGP neighbor, and the OSPF route will further depend on a connected route to resolve the nexthop ip address to an output interface.
%\begin{figure}[h]
 \begin{minted}[breaklines,linenos,fontsize=\small]{python}
def infer_main_route_recursive(r, input_facts):
  rib = input_facts.main_rib_entries.lookup(
    host=r.host
  )
  current_route = r
  inferred_edges = []
  while is_ipaddress(current_route.nexthop):
    nh_resolution_route = longest_prefix_match(
      input_rib=rib,
      ip=current_route.nexthop
    )
    inferred_edges.append((current_route, nh_resolution_route))
    current_route = nh_resolution_route
  return inferred_edges
 \end{minted}
%\caption{Infer RIB entries that led to a FIB entry.}
%\end{figure}
 
\para{Dependencies of a post-import BGP message is a mini-graph} A post-import BGP message is derived by applying import policy on the pre-import message. We compute pre-import message on-the-fly by simulating BGP export using another policy evaluation. Policy evaluations also reports the policy terms exercised during the process, which are also the dependencies of derived messages.
%\begin{figure}[h]
 \begin{minted}[breaklines,linenos,fontsize=\small]{python}
def infer_bgp_message(m, input_facts):
  bgp_edge = input_facts.bgp_edges.lookup(
    recv_host=m.host
    send_ip=m.nexthop
  )
  grandparent_route = input_facts.bgp_rib_entries.lookup(
    host=bgp_edge.send_host,
    prefix=r.prefix,
    status='BEST'
  )
  parent_message, export_terms = policy_evaluation(
    input_route=grandparent_route,
    policy=bgp_edge.export_policy
  )
  _, import_terms = policy_evaluation(
    input_route=parent_message,
    policy=bgp_edge.import_policy
  )
  return [
    (m, parent_message),
    (m, bgp_edge)
    *[(m, term) for term in import_terms],
    (parent_message, grandparent_route),
    (parent_message, bgp_edge),
    *[(parent_message, term) for term in export_terms]
  ]
 \end{minted}
%\caption{Infer RIB entries that led to a FIB entry.}
%\end{figure}

\para{BGP edge from BGP peer configurations} 
%\begin{figure}[h]
 \begin{minted}[breaklines,linenos,fontsize=\small]{python}
def infer_edge_from_peer_config(e, input_facts):
  send_config = input_facts.bgp_peer_configs.lookup(
    host=e.send_host
    remote_as=e.recv_as
    remote_ip=e.recv_ip
  )
  recv_config = input_facts.bgp_peer_configs.lookup(
    host=e.recv_host
    remote_as=e.send_as
    remote_ip=e.send_ip
  )
  return [(e, send_config), (e, recv_config)]
 \end{minted}
%\caption{Infer RIB entries that led to a FIB entry.}
%\end{figure}

\para{BGP edge from data plane path} 
%\begin{figure}[h]
 \begin{minted}[breaklines,linenos,fontsize=\small]{python}
def infer_edge_from_path(e, input_facts):
  forward_path = IFGNode(
    type='path',
    send_host=e.send_host,
    recv_host=e.recv_host,
    send_ip=e.send_ip,
    recv_ip=e.recv_ip,
    send_port=179,
    recv_port=179,
    ip_protocol='TCP'
  )
  backward_path = IFGNode(
    type='path',
    send_host=e.recv_host,
    recv_host=e.send_host,
    send_ip=e.recv_ip,
    recv_ip=e.send_ip,
    send_port=179,
    recv_port=179,
    ip_protocol='TCP'
  )
  return [(e, forward_path), (e, backward_path)]
 \end{minted}
%\caption{Infer RIB entries that led to a FIB entry.}
%\end{figure}

\para{Infer exercised main RIB entries and ACL entries for a data plane path} 
%\begin{figure}[h]
 \begin{minted}[breaklines,linenos,fontsize=\small]{python}
def infer_path_from_main_route(p, input_facts):
  exercised_routes, exercised_acls = traceroute(
    start_location=p.send_host,
    src_ip=p.send_ip,
    dst_ip=p.recv_ip,
    src_port=p.send_port,
    dst_port=p.recv_port,
    ip_protocol=p.ip_protocol
  )
  return [
    *[(p, route) for route in exercised_routes],
    *[(p, acl) for acl in exercised_acls]
  ]
 \end{minted}
%\caption{Infer RIB entries that led to a FIB entry.}
%\end{figure}
