# Supplementary material for: Test Coverage for Network Configurations
Source: arXiv:2209.12870 source file (2022-09-26)
Supplement: Supplementary file 5 [file old.tex]

\para{FIB entry from main RIB route} The following code shows the inference rule to infer RIB entries from FIB entry. Based on control plane semantics, each FIB entry is computed by selecting the best route of its prefix in the same router's RIB and resolving the forwarding interface based on the best route's next hop IP address. \xieyang{model the second one with ARP table?} %Line 2-7 computes the best route by first looking up all entries in the same router's RIB with the same prefix as the FIB entry, and then select the one with the lowest administrative distance. Line 8-12 computes the route used for IP resolution. It looks up all rib entries on the router and select the one with longest prefix matching.
%\begin{figure}[h]
 \begin{minted}[breaklines,linenos,fontsize=\small]{python}
def infer_fib_entry_from_main_route(f, input_facts):
  rib = input_facts.lookup(
    type='rib_entry',
    host=f.host
  )
  best_route = best_route_selection(
    input_rib=rib,
    prefix=f.prefix
  )
  ip_resolution_route = longest_prefix_match(
    input_rib=rib,
    ip=best_route.nexthop
  )
  return [best_route, ip_resolution_route]
 \end{minted}
%\caption{Infer RIB entries that led to a FIB entry.}
%\end{figure}

\para{Map BGP route to }
%\begin{figure}[h]
 \begin{minted}[breaklines,linenos,fontsize=\small]{python}
def infer_bgp_route_from_message(r, input_facts):
  bgp_edge = input_facts.lookup(
    type='bgp_edge',
    recv_host=r.host
    send_ip=r.nexthop
  )
  grandparent_route = input_facts.lookup(
    type='bgp_rib_entry',
    host=bgp_edge.send_host,
    prefix=r.prefix,
    status='BEST'
  )
  parent = bgp_export_simulation(
    input_route=grandparent_route,
    bgp_edge=bgp_edge
  )
  return [(r, parent), (parent, bgp_edge), (parent, grandparent_route)]
 \end{minted}
%\caption{Infer RIB entries that led to a FIB entry.}
%\end{figure}

\para{BGP message from BGP edge}
%\begin{figure}[h]
 \begin{minted}[breaklines,linenos,fontsize=\small]{python}
def infer_message_from_edge(m, input_facts):
  bgp_edge = input_facts.lookup(
    type='bgp_edge',
    recv_host=m.recv_host
    send_host=m.send_host
  )
  return [bgp_edge]
 \end{minted}
%\caption{Infer RIB entries that led to a FIB entry.}
%\end{figure}

\para{BGP message from BGP route at sender}
%\begin{figure}[h]
 \begin{minted}[breaklines,linenos,fontsize=\small]{python}
def infer_message_from_bgp_route(m, input_facts):
  parent = input_facts.lookup(
    type='bgp_rib_entry',
    host=m.send_host,
    prefix=m.prefix,
    status='BEST'
  )
  return [parent]
 \end{minted}
%\caption{Infer RIB entries that led to a FIB entry.}
%\end{figure}

\para{BGP message from routing policy terms} TRP requires information from two other parents of the message fact--BGP edge and the BGP route in sender's BGP RIB. To discover them, this rule leverages two other rules defined above.
%\begin{figure}[h]
 \begin{minted}[breaklines,linenos,fontsize=\small]{python}
def infer_message_from_export_policy(m, input_facts):
  bgp_edge = infer_message_from_edge(m, input_facts)
  parent_route = infer_message_from_bgp_route(m, input_facts)
  terms = test_routing_policy(
    input_route=parent_route,
    policy=bgp_edge.export_policy
  )
  return [*terms]
 \end{minted}
%\caption{Infer RIB entries that led to a FIB entry.}
%\end{figure}

\begin{figure}
 \begin{minted}[breaklines,linenos,fontsize=\small]{python}
class MainRibFromBgpRib(InferenceRule):
  def is_applicable(r):
    return r.type=='main_rib_entry' and r.protocol=='bgp'
  def infer(r, input_facts):
    parent = input_facts.bgp_rib_entries.lookup(
      host=r.host,
      prefix=r.prefix,
      nexthop=r.nexthop,
      status='BEST'
    )
    return [(r, parent)]
 \end{minted}
\caption{An example inference rule. \py{is_applicable} function is a predicate for whether the input IFG node falls in the rule's domain. \py{infer} function implements the rule's inference logic, whose return value is a list of \py{(child, parent)} tuples denoting inferred edges. \xieyang{Is \py{status} a Batfish-specific attribute or a generic control plane attribute?}}
\label{fig:infer_main_from_bgp}
\end{figure}

\begin{figure}
 \begin{minted}[breaklines,linenos,fontsize=\small]{python}
class BgpMsgFromPolicyEvaluation(InferenceRule):
  def is_applicable(m):
    return m.type=='bgp_message' and m.status=='post_import'
  def infer(m, input_facts):
    bgp_edge = input_facts.bgp_edges.lookup(
      recv_host=m.recv_host,
      send_host=m.send_host,
      send_ip=m.nexthop_ip
    )
    grandparent_route = input_facts.bgp_rib_entries.lookup(
      host=m.send_host,
      prefix=m.prefix,
      status='BEST' # TODO:may not be unique for ECMP
    )
    parent_message, export_terms = policy_evaluation(
      input_route=grandparent_route,
      policy=bgp_edge.export_policy
    )
    _, import_terms = policy_evaluation(
      input_route=parent_message,
      policy=bgp_edge.import_policy
    )
    return [
      (m, parent_message),
      (m, bgp_edge)
      *[(m, term) for term in import_terms],
      (parent_message, grandparent_route),
      (parent_message, bgp_edge),
      *[(parent_message, term) for term in export_terms]
    ]
 \end{minted}
\caption{An example inference rule that combines lookup-based backward inference and simulation-based forward inference.}
\label{fig:infer_bgp_from_message}
\end{figure}

\begin{algorithm}[!ht]
\footnotesize
\DontPrintSemicolon
  \SetKwFunction{Infer}{InferBgpRibFromMainRib}
  \SetKwProg{myproc}{Procedure}{}{}
  \KwInput{IFG node $v$}
  %\KwOutput{IFG edges $\{(u, v)\}$}
  \KwData{BGP RIB $\mathcal{R}_{bgp}$}
  
    \myproc{\Infer{$v$}}
    {
        \If{\upshape $v$ is $\textsc{MainRibEntry} \wedge protocol_{v}=bgp$}
        {
            $u \leftarrow \textsc{lookup}(\mathcal{R}_{bgp}@host_v,~ prefix_v,~ nexthop_v,~ 1) \in $\;
            \Return $\{(u, v)\}$
        }
        \Else
        {
            \Return $\{\}$
        }
    }
\caption{Infer $f_i \leftarrow r_j$ \label{alg:main-from-bgp}}
\end{algorithm}

We model the criticalness between facts with logical necessity. We represent the condition of whether a fact is valid using a Boolean predicate $\Gamma$. The validity of a fact depends on the validity of its ancestors in the IFG. A normal node depends on the conjunction of its immediate parents; A disjunctive node depends on the disjunction of parents; A configuration fact does not have parents, so we represent its validity as a Boolean variable:
\begin{equation}
    \Gamma(v) = 
    \begin{cases}
      \bigvee_{u \in \texttt{pred}(v)} \Gamma(u) & \text{if}~v~\text{is a disjunctive node} \\
      x_i & \text{if}~v~\text{denotes configuration fact}~c_i\\
      \bigwedge_{u \in \texttt{pred}(v)} \Gamma(u) & \text{otherwise}
    \end{cases}
    \label{eq:causal_dependency}
\end{equation}
Therefore the validity of any IFG node ultimately depends on the validity of configuration elements that lead to it, denoted as $\Gamma(v)=F(x_1, \dots, x_n)$. Formally, a configuration element $c_i$ is critical to fact $v$ iff its validity, denoted as $x_i$, is necessary for the validity of $v$:
\[
\neg x_i \to \neg \Gamma(v)
\]


We determine if a configuration element is weakly covered as follows. The validity of IFG nodes are represented as BDD (for binary decision diagrams) predicates. We perform a post-order traversal to build BDD predicates bottom-up, following \autoref{eq:causal_dependency}. Once the predicates are built, we test graph reachability and necessity between each pair of configuration facts and tested facts. Necessity $\neg x_i \rightarrow \neg \Gamma(v)$ is equivalent to unsatisfactory of $\neg x_i \wedge \Gamma(v)$. While (un)satisfactory is NP-Complete in general cases, we note that it is efficient in our case---it can be reduced to computing cofactor ($\Gamma(v)|_{x_i=0}=F_{x_i'}$) and testing whether the cofactor is constant false, both of which are efficient using BDD operations.

\begin{algorithm}[!h]
\footnotesize
\DontPrintSemicolon
  \SetKwProg{Infer}{Infer}{}{}
  \SetKwFunction{Infer}{Infer}
  \SetKwProg{myproc}{Procedure}{}{}
  \KwInput{IFG node $v=\textsc{BgpMsg}(sh, rh, p, nh, (a_i), \{cm_i\}, pi)$}
  %\KwOutput{IFG edges $\{(u, v)\}$}
  \KwData{BGP RIB $\mathcal{R}_{bgp}=\{\textsc{BgpRoute}(h, p, nh, (a_i), \{cm_i\}, lp, b)\}$, \hspace{30pt} BGP edges $\mathcal{E}_{bgp}=\{\textsc{BgpEdge}(sh, rh, si, ri, sa, ra, ep, ip)\}$}
  
    \myproc{\Infer{$v$}}
    {
        \If{\upshape $v$ is $\textsc{BgpMsg} \wedge pi_{v}=0$} 
        {
            %$E \leftarrow \varnothing$ \;
            $w \leftarrow \textsc{lookup}(h=sh_v, ~p=p_v, ~b=1) \in \mathcal{R}_{bgp}$\;
            $e \leftarrow \textsc{lookup}(sh=sh_v, ~rh=rh_v, ~si=nh_v, ~sa=a_{1_v}) \in \mathcal{E}_{bgp}$  \tcp*{$a_{1_v}$ is 1st element of $(a_i)_v$}
            $(u, \{c_i\}_{ep}) \leftarrow \textsc{eval}(policy=ep_e, route=w)$\;
            $(v', \{c_i\}_{ip}) \leftarrow \textsc{eval}(policy=ip_e, route=u)$\;
            %$E \leftarrow E \cup \{()\}$\;
            \Return $\{(u, v), (e, v)\} \cup \{(c_i, v) \mid c_i \in \{c_i\}_{ep}\} \cup \{(w, u), (e, u)\} \cup \{(c_i, u) \mid c_i \in \{c_i\}_{ip}\}$
        } 
        \Else
        {
            \Return $\{\}$
        }
    }
\caption{Infer dependencies of $\textsc{BgpMsg}$ \label{alg:bgp-message}}
\end{algorithm}

\section{Introduction} \label{sec:introduction} 

%\brief{The need of network configuration verification.}

Correct network configurations are critical to network security and reliability. However, it is known to be hard and error-prone to create and maintain configurations for the network. Configurations are comprised of vendor-specific commands to manipulate complicated routing protocols running distributedly over the network. Moreover, networks are complex and their configurations are built incrementally with small operational updates over the years. It is extremely hard to judge the correctness of network configurations even for experienced network engineers. As a result, misconfiguration has been a major cause of network outages \cite{twitter, level3misconfiguration, azuremisconfiguration, cloudflaremisconfiguration} and leads to significant consequences. Within the past single year, the For example, both Facebook \cite{fboutage} and Cloudflare \cite{xx} suffered 

To battle this challenge, testing and verification of network configurations have surged in both the academia and industry, and have been adopted by all major cloud providers \cite{aws-inspector, rcdc, houyan}. %\todo{add reference to testing} 
These testing/verification frameworks can 
However, as we learnt from helping deploy verification for multiple networks, \textit{outages can still happen} when the test suites used are incomplete and leave some blind spots of the configurations untested.

A glib suggestion to this problem is that network engineers should develop better test suites, but that is easier said than done. Due to the complexity of the network and its configurations, it can be nearly impossible for an engineer to judge how good a test suite is and what it does not test. Network engineers need better tools to make these judgements.

We draw inspiration from software testing to create such tools. The software domain has a range of coverage metrics that quantify the quality of test suites and provide insight into what aspects of the software are not well covered~\cite{sw-book-myers,sw-book-amman}. Systems that compute and report coverage metrics are now an integral part of any software testing platform~\cite{google-coverage, vs-coverage, codecov}.

In networking, coverage metrics have recently been introduced for stateless network data planes \cite{yardstick}. Data plane metrics quantify how well different data plane components such as forwarding rules are exercised and they support a range of test types. However, data plane metrics are inadequate for the verification of configurations (also known as control plane verification) for two reasons. First, the data plane is the output of control plane; High coverage of the output does not necessarily reflect high coverage of the input. Second, the derived data plane is a function of input configuration as well as the network \textit{environment}, which includes the up/down status of links in the network and routing information coming in from outside of the network. The comprehensiveness of control plane verification should be evaluated among all possible environments, while the data plane metrics are limited to single fixed environment. Therefore, we need coverage metrics specialized for network configurations.

A major challenge that we face is to track implicit mapping from directly tested facts back to components of configurations. Unlike software or data plane, the tests of control plane verification does not directly execute or exercise its input, \IE, lines or blocks of configurations. Instead, the configurations are first used to produce the data planes, and the tests run on top of the data plane facts. To know which configuration lines are tested, we need to know which lines have participated in the derivation of tested data plane facts.

We propose to track and compute such mapping by modeling the network as a dependency graph. Each configuration block or data plane route is a node of the graph, and directed edges are used to model the dependencies between nodes. A node n1 is a derived (child) node of another node n2 if the derivation of n1 depends on the existence of n2 or leverages any information contained by n2. And thus, if a derived node is covered, all of its parent nodes are covered, albeit indirectly. With the help of dependency graph, the mapping problem can be reduced to simple graph traversal problems. The formulation of our network dependency graph is also tuned to achieve scalability and to support different granularity. Our model focuses on the converged state instead of transient state of network to avoid overhead on unnecessary graph branches. Many configuration structures are hierarchical and can be modeled at different granularity. We achieve efficient representation and dependency tracking of such configuration structure at any granularity by chaining them with intermediate nodes and compute the unrolling on demand.

We build a system to compute configuration coverage based on this framework. It does not require any instrumentation inside the verification tools or any tracing during the run time of tests. It computes tested graph nodes from test result returned by the verification tool, and lazily construct a minimal subset of the dependency graph to find the set of covered configurations. It uses a novel ``retroduction-and-match'' algorithm that leverages domain-specific heuristics and partial information provided by verification tools.

To demonstrate the value of configuration coverage, we present a case study where configuration coverage is compared side-by-side with data plane coverage for a set of test suites. We also benchmark the performance of our system using synthetic data center networks of varying sizes. We find that in addition to the zero overhead on test execution, it is fast to compute configuration coverage after the tests are done. The worst case time consumption is 438 seconds, which is less than 15\% compared to the test execution itself.

\begin{algorithm}[!t]
\footnotesize
\DontPrintSemicolon\SetAlgoNoEnd\SetAlgoNoLine
  \SetKwFunction{Infer}{InferBgpRibFromMainRib}
  \SetKwProg{myproc}{}{}{}
    \myproc{\Infer{$f$}}
    {
        \If{\upshape $f$ \textbf{is not} $\textsc{MainRibEntry}$ \textbf{or} $f.protocol \neq bgp$}
        {
            \Return $\{\}$
        }
        $r = \textsc{lookupBgpRib}(@f.host, f.prefix, f.nexthop)$\;
        \Return $\{(r, f)\}$
    }
\caption{Rule to infer BGP RIB entry from main RIB entry \label{alg:main-from-bgp}}
\end{algorithm}

\begin{algorithm}[!t]
\footnotesize
\DontPrintSemicolon
  \SetKwFunction{Infer}{Infer}
  \SetKwProg{myproc}{Procedure}{}{}

    \myproc{\Infer{$m$}}
    {
        \If{\upshape $m$ \textbf{is not} $\textsc{BgpMsg}$ \textbf{or} $m.is\_pre\_import=1$} 
        {
            \Return $\{\}$
        } 
        %$E \leftarrow \varnothing$ \;
        $r \leftarrow \textsc{lookupBgpRib}(@m.send\_host, m.prefix)$\;
        $e \leftarrow \textsc{lookupBgpEdge}(@m.send\_host, m.recv\_host,$  $m.nexthop, m.as\_path[0])$ \;
        $(m', \{c_i\}_{ep}) \leftarrow \textsc{simPolicyEval}(e.export\_policy, r)$\;
        $(m'', \{c_i\}_{ip}) \leftarrow \textsc{simPolicyEval}(e.import\_policy, m')$\;
        %$E \leftarrow E \cup \{()\}$\;
        \Return $\{(m', m), (e, m)\} \cup \{(c_i, m) \mid c_i \in \{c_i\}_{ep}\} \cup \{(r, m'), (e, m')\} \cup \{(c_i, m') \mid c_i \in \{c_i\}_{ip}\}$
    }
\caption{Rule to infer parents of a post-import BGP message
\label{alg:bgp-message}}
\end{algorithm}

\begin{algorithm}[t]
\footnotesize
\DontPrintSemicolon
  \SetKwFunction{BuildIFG}{BuildIFG}
  \SetKwProg{myproc}{Procedure}{}{}
  \KwInput{Initial nodes $\{v_i\}$; Inference rules $\{\phi_i: v \mapsto \{(u_i, v_i)\}\}$;}
  \KwOutput{Materialized IFG $(V, E)$}
  \KwData{Stable state data plane state (main RIB and protocol RIBs);
    Routing edges; Configuration elements; Environment;}
  
    \myproc{\BuildIFG{$\{v_i\}$, $\{\phi_i\}$}}
    {
        $V, E \leftarrow \{v_i\}, \varnothing$ \;
        $V' \leftarrow \{v_i\}$ \tcp*{dirty nodes of previous iteration}
        \While{$|V'| > 0$}
        {
            $V'' \leftarrow \varnothing$ \tcp*{dirty nodes of current iteration}
            \ForEach{$c \in V'$}
            {
                \ForEach{$\phi \in \{\phi_i\}$}
                {
                    $E' \leftarrow \phi(c)$ \;
                    \ForEach{$(u_i, v_i) \in E'$}
                    {
                        \If{$u_i \notin V$}
                        {
                            $V \leftarrow V \cup \{u_i\}$,
                            $V'' \leftarrow V'' \cup \{u_i\}$
                        }
                        \If{$v_i \notin V$}
                        {
                            $V \leftarrow V \cup \{v_i\}$,
                            $V'' \leftarrow V'' \cup \{v_i\}$
                        }
                        \lIf{$(u_i, v_i) \notin E$}
                        {
                            $E \leftarrow E \cup \{(u_i, v_i)\}$
                        }
                    }
                }
            }
            $V' \leftarrow V''$\;
        }
        \Return{$(V, E)$}
    }
\caption{IFG lazy materialization}\label{alg:ifg-materialization}
\end{algorithm}
